# Supplementary material for: Reinforcement Learning in Factored Action Spaces using Tensor Decompositions
Source: arXiv:2110.14538 source file (2021-10-27)
Supplement: Supplementary file 1 [file appendix_experiments.tex]

\section{Additional experiments and details}
\label{app:additional_exp}

\subsection{StarCraft II}
\label{app:sc2}
\begin{figure}[h]
% \begin{wrapfigure}{r}{0.4\textwidth}
    \centering
    %\vspace{-0.2cm}
    \includegraphics[width=0.4\linewidth]{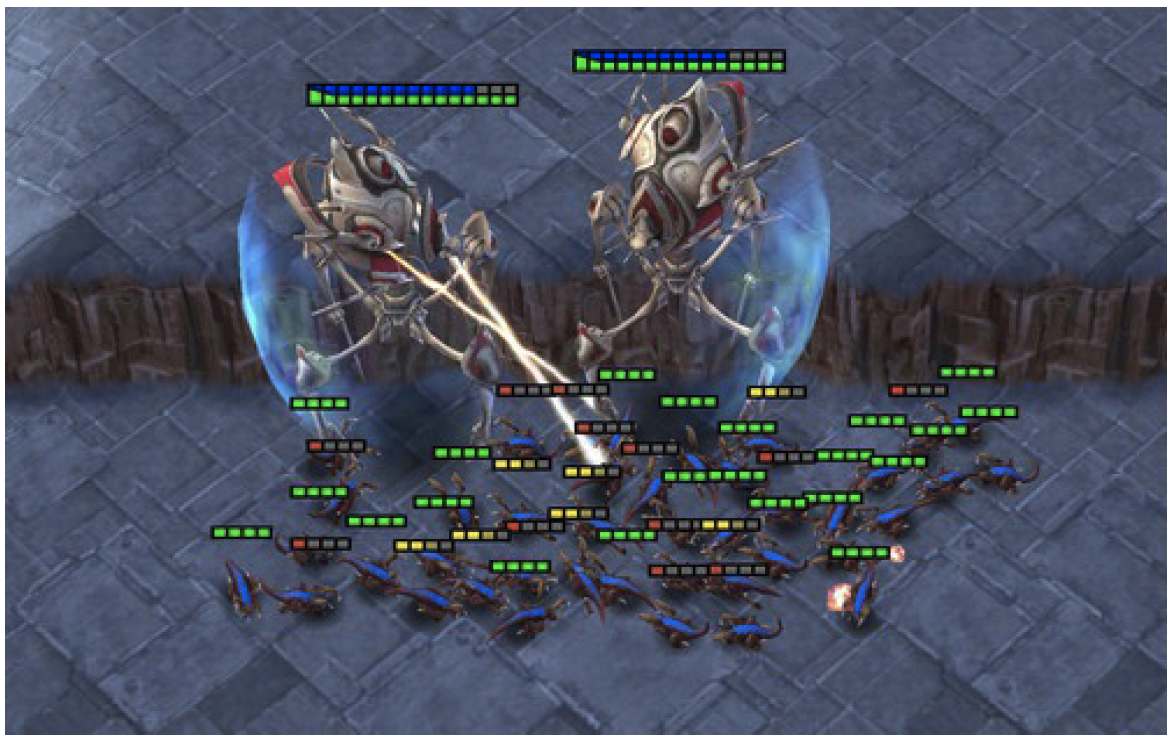}
    \caption{The 2c\_vs\_64zg scenario in SMAC. \label{fig:snap_col}}
%    \vspace{-0.3cm}
% \end{wrapfigure}
\end{figure}

In the SMAC bechmark\citep{samvelyan2019starcraft} (https://github.com/oxwhirl/smac), agents can $\mathtt{move}$ in four cardinal directions, $\mathtt{stop}$, take $\mathtt{noop}$ (do nothing), or select an enemy to $\mathtt{attack}$ at each timestep. Therefore, if there are $n_e$ enemies in the map, the action space for each ally unit contains $n_e + 6$ discrete actions. 
\subsubsection{Additional Experiments}
\label{app:additional_sc2}
\begin{figure*}[h]
	\centering
	\subfigure[3s5z \textbf{Easy}]{
		\includegraphics[width=0.325\linewidth]{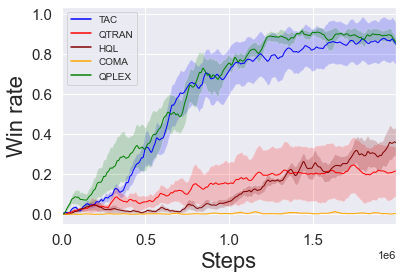}\label{fig:a_3s5z_smac}}
	\subfigure[2s\_vs\_1sc \textbf{Easy}]{
		\includegraphics[width=0.325\linewidth]{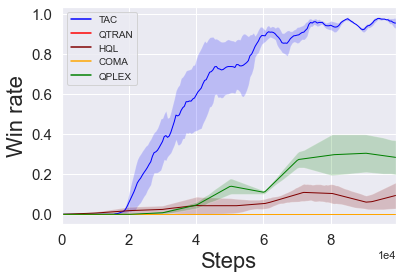}\label{fig:a_2s_vs_1sc}}
	\subfigure[2c\_vs\_64zg \textbf{Hard}]{
		\includegraphics[width=0.325\linewidth]{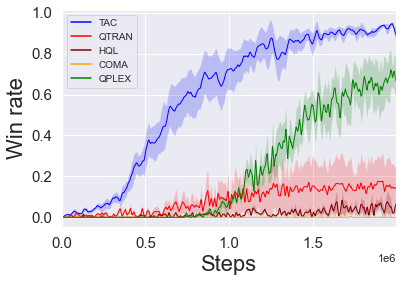}\label{fig:a_2c_vs_64z}}
% 	\vspace{-2mm}
	\subfigure[5m\_vs\_6m \textbf{Hard}]{
		\includegraphics[width=0.325\linewidth]{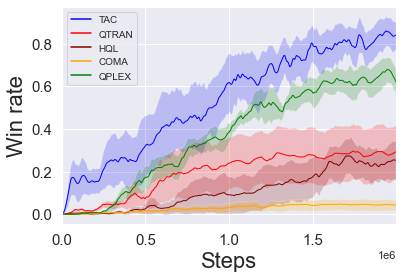}\label{fig:a_5m_vs_6m}}
	\subfigure[MMM2 \textbf{Super Hard}]{
		\includegraphics[width=0.325\linewidth]{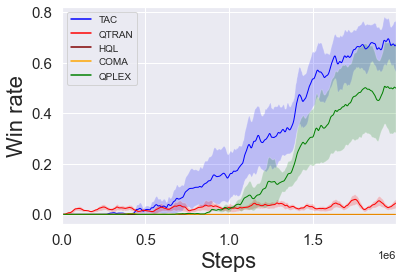}\label{fig:a_MMM2}}
	\subfigure[27m\_vs\_30m \textbf{Super Hard}]{
		\includegraphics[width=0.325\linewidth]{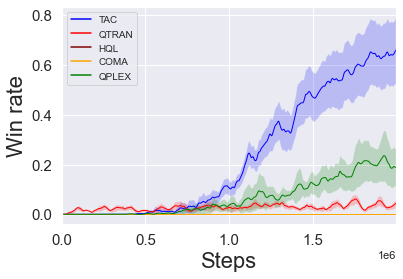}\label{fig:a_27m_vs_30m}}
% 	\vspace{-2mm}
	\subfigure[6h\_vs\_8z \textbf{Super Hard}]{
		\includegraphics[width=0.325\linewidth]{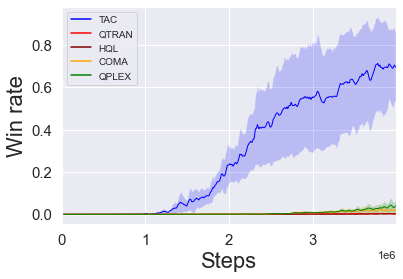}\label{fig:a_6h8z}}
	\subfigure[Corridor \textbf{Super Hard}]{
		\includegraphics[width=0.325\linewidth]{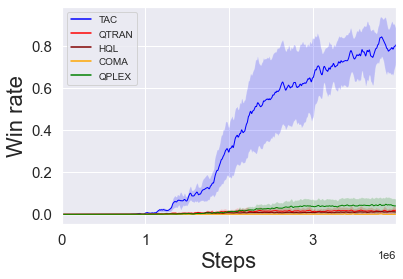}\label{fig:a_corridor}}
% 	\vspace{-3mm}
	\caption{Performance of different algorithms on different SMAC scenarios: \textcolor{blue}{TAC}, \textcolor{red}{QTRAN}, \textcolor[rgb]{0,0.7,0}{QPLEX}, \textcolor{orange}{COMA}, \textcolor[rgb]{0.76, 0.13, 0.28}{HQL}. \label{fig:additional_sc2}}
% 	\vspace{-3mm}
\end{figure*}

In addition to the baselines in main text \cref{sec:exps}, we also include 4 more baselines: \textcolor{red}{QTRAN} \citep{son2019qtran}, \textcolor[rgb]{0,0.7,0}{QPLEX} \citep{wang2020qplex}, \textcolor{orange}{COMA} \citep{foerster2018counterfactual} and \textcolor[rgb]{0.76, 0.13, 0.28}{HQL}. QTRAN tries to avoid the issues arising with representational constraints by posing the decentralised multi agent problem as optimisation with linear constraints, these constraints are relaxed using L2 penalties for tractability \citep{mahajan2019maven}. Similarly, QPLEX another recent method uses an alternative formulation using advantages for ensuring the \textit{Individual Global Max} (IGM) principle \citep{son2019qtran}. COMA is an actor-critic method that uses a centralised critic for computing a counterfactual baseline for variance reduction by marginalising across individual agent actions. Finally, HQL uses the heuristic of differential learning rates on top of IQL \citep{tan_multi-agent_1993} to address problems associated with decentralized exploration. \textbf{\cref{fig:additional_sc2} }gives the average win rates of the baselines on different SMAC scenarios across five random runs (with one standard deviation shaded). We observe that \textsc{Tesseract} outperforms the baselines by a large margin on most of the scenarios, especially on the \textbf{super-hard} ones on which the exiting methods struggle, this validates the sample efficiency and representational gains supported by our analysis. We observe that HQL is unable to learn a good policy on most scenarios, this might be due to uncertainty in the bootstrap estimates used for choosing the learning rate that confounds with difficulties arising from non-stationarity. We also observe that COMA does not yield satisfactory performance on any of the scenarios. This is possibly because it does not utilise the underlying tensor structure of the problem and suffers from a \textit{lagging critic}. While QPLEX is able to alleviate the problems arising from relaxing the IGM constraints in QTRAN, it lacks in performance on the \textbf{super-hard} scenarios of Corridor and 6h\_vs\_8z. 

\subsubsection{Experimental Setup for SMAC}
\label{app:setup_sc2}
We use a factor network for the tensorised critic which comprises of a fully connected MLP with two hidden layers of dimensions 64 and 32 respectively and outputs a $r|U|$ dimensional vector. We use an identical policy network for the actors which outputs a $|U|$ dimensional vector and a value network which outputs a scalar state-value baseline $V(s)$. The agent policies are derived using softmax over the policy network output. Similar to previous work \cite{samvelyan2019starcraft}, we use two layer network consisting of a fully-connected layer followed by GRU (of 64-dimensional hidden state) for encoding agent trajectories. We used Relu for non-linearities. All the networks are shared across the agents. We use ADAM as the optimizer with learning rate $5\times10^{-4}$. We use entropy regularisation with scaling coefficient $\beta = 0.005$. We use an approximation rank of $7$ for Tesseract ('TAC') for the SMAC experiments. A batch size of 512 is used for training which is collected across 8 parallel environments (additional setup details in \cref{app:techniques}). Grid search was performed over the hyper-parameters for tuning. 

For the baselines QPLEX, QMIX, QTRAN, VDN, COMA, IQL we use the open sourced code provided by their authors at https://github.com/wjh720/QPLEX and https://github.com/oxwhirl/pymarl respectively which has hyper-parameters tuned for SMAC domain. The choice for architecture make the experimental setup of the neural networks used across all the baselines similar. We use a similar trajectory embedding network as mentioned above for our implementations of HQL and FQL which is followed by a network comprising of a fully connected MLP with two hidden layers of dimensions 64 and 32 respectively. For HQL this network outputs $|U|$ action utilities. For FQL, it outputs  a $|U|+d$ vector: first $|U|$ dimension are used for obtaining the scalar contribution to joint Q-function and rest $d$ are used for computing interactions between agents via inner product. We use ADAM as the optimizer for these two baselines. We use differential learning rates of $\alpha = 1\times10^{-3}, \beta=2\times10^{-4}$ for HQL searched over a grid of $\{1,2,5,10\}\times10^{-3} \times\{1,2,5,10\}\times10^{-4}$. FQL uses the same learning rate $5\times10^{-4}$ with $d = 10$ which was  searched over set $\{5, 10, 15\}$. 

The baselines use $\epsilon-$greedy for exploration with $\epsilon$ annealed from $1.0 \to 0.05$ over 50K steps. For super-hard scenarios in \textbf{SMAC} we extend the anneal time to 400K steps. We use temperature annealing for \textsc{Tesseract} with temperature given by $\tau = \frac{2T}{T+t}$ where $T$ is the total step budget and $t$ is the current step. Similarly we use temperature $\tau = \frac{4T}{T+3t}$ for super-hard \textbf{SMAC} scenarios. The discount factor was set to $0.99$ for all the algorithms. 

Experiment runs take 1-5 days on a Nvidia DGX server depending on the size of the StarCraft scenario.

\subsection{Techniques for stabilising \textsc{Tesseract} critic training for Deep-MARL}
\label{app:techniques}
\begin{itemize}
    \item We used a gradient normalisation of $0.5$. The parameters exclusive to the critic were separately subject to the gradient normalisation, this was done because the ratio of gradient norms for the actor and the critic parameters can vary substantially across training. 
    \item We found that using multi-step bootstrapping substantially reduced target variance for Q-fitting and advantage estimation (we used the advantage based policy gradient $\int_{S} \rho^\pi(s)\int_{\mathbf{U}}\nabla\pi_\theta(\mathbf{u|s})\hat A^{\pi}(s,\mathbf{u}) d\mathbf{u}ds$ \citep{sutton2011reinforcement}) for \textbf{SMAC} experiments. Specifically for horizon T, we used the Q-target as:
    \begin{align}
        &Q_{target,t} = \sum_{k=1}^{T-t} \lambda^{k}g_{t,k} \\
        & g_{t,k} = R_t + \gamma R_{t+1} + ... + \gamma^{k}V(s_{t+k}) 
    \end{align}

    and similarly for value target. Likewise, the generalised advantage is estimated as:
    \begin{align}
        &\hat A_t = \sum_{k=0}^{T-t} (\gamma\lambda)^{k}\delta_{t+k}\\
        &\delta_{t} = R_{t}+ \gamma\hat Q(s_{t+1}, \mathbf{u}_{t+1})-V(s_t)
    \end{align}

    Where $\hat Q$ is the tensor network output and the estimates are normalized by the accumulated powers of $\lambda$. We used $T=64, \gamma = 0.99$ and $\lambda = 0.95$ for the experiments.
    \item The tensor network factors were squashed using a sigmoid for clipping and were scaled by $2.0$ for \textbf{SMAC} experiments. Additionally, we initialised the factors according to $\mathcal{N}(0, 0.01)$ (before applying a sigmoid transform) so that value estimates can be effectively updated without the gradient vanishing.
    \item  Similarly, we used clipping for the action-value estimates $\hat Q$ to prevent very large estimates:
    \begin{align}
    clip(\hat{Q}_t) = min\{\hat{Q}_t, R_{max}\}
    \end{align}
    we used $R_{max}=40$ for the \textbf{SMAC} experiments.
\end{itemize}

\begin{figure*}[h]
	\centering
	\subfigure[Ablation on stabilisation techniques]{
		\includegraphics[width=0.4\linewidth]{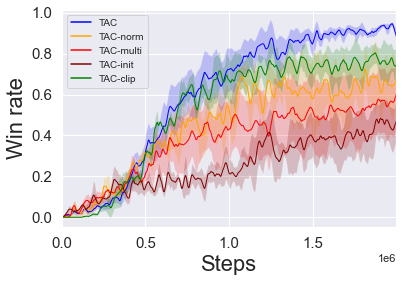}\label{fig:ab_tech}}
	\subfigure[Ablation on rank]{
		\includegraphics[width=0.4\linewidth]{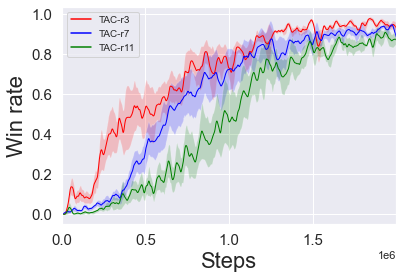}\label{fig:ab_rank}}
	\caption{Variations on \textsc{Tesseract} \label{fig:ablation_sc2}}
% 	\vspace{-3mm}
\end{figure*}
We provide the ablation results on the stabilisation techniques mentioned above on the 2c\_vs\_64zg scenario in \cref{fig:ab_tech}. The plot lines correspond to the ablations: \textcolor{red}{TAC-multi}: no multi-step target and advantage estimation, \textcolor[rgb]{0,0.7,0}{TAC-clip}: no value upper bounding/clipping, \textcolor{orange}{TAC-norm}: no separate gradient norm, \textcolor[rgb]{0.76, 0.13, 0.28}{TAC-init}: no initialisation and sigmoid squashing of factors. We observe that multi-step estimation of target and advantage plays a very important role in stabilising the training, this is because noisy estimates can adversely update the learn factors towards undesirable fits. Similarly, proper initialisation plays a very important role in learning the Q-tensor as otherwise a larger number of updates might be required for the network to learn the correct factorization, adversely affecting the sample efficiency. Finally we observe that max-clipping and separate gradient normalisation do impact learning, although such effects are relatively mild. 

We also provide the learning curves for \textsc{Tesseract} as the CP rank of Q-approximation is changed, \cref{fig:ab_rank} gives the learning plots as the CP-rank is varied over the set $\{3, 7, 11\}$. Here, we observe that approximation rank makes little impact on the final performance of the algorithm, however it may require more samples in learning the optimal policy. Our PAC analysis \cref{thm:debound} also supports this. 

\subsection{Tensor games:} 
\label{app:tg}
We introduce tensor games for our experimental evaluation. These games generalise the matrix games often used in $2$-player domains. Formally, a tensor game is a cooperative MARL scenario described by tuple $(n,|U|,r)$ that respectively defines the number of agents (dimensions), the number of actions per agent (size of index set) and the rank of the underlying reward tensor \cref{fig:tgg}. Each agent learns a policy for picking a value from the index set corresponding to its dimension. The joint reward is given by the entry  corresponding to the joint action picked by the agents, with the goal of finding the tensor entry corresponding to the maximum reward. We consider the CTDE setting for this game, which makes it additionally challenging. We compare \textsc{Tesseract} (\textcolor{blue}{TAC}) with \textcolor[rgb]{0,0.7,0}{VDN}, \textcolor{red}{QMIX} and independent actor-critic (\textcolor[rgb]{0.76, 0.13, 0.28}{IAC})  trained using Reinforce \cite{sutton2000policy}. Stateless games provide are ideal for isolating the effect of an exponential blowup in the action space. The natural difficulty knobs for stateless games are $|n|$ and $|U|$ which can be increased to obtain environments with  large joint action spaces. Furthermore, as the rank $r$ increases, it becomes increasingly difficult to obtain good approximations for $\hat T$.

 \begin{figure}[h]
%\begin{wrapfigure}{r}{0.4\textwidth}
    \centering
    %\vspace{-0.2cm}
    \includegraphics[width=0.33\linewidth]{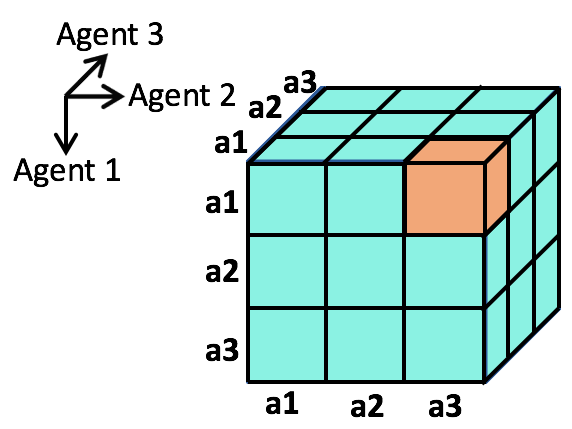}
    \caption{Tensor games example with $3$ agents ($n$) having $3$ actions each ($a$). Optimal joint-action \textbf{(a1, a3, a1)} shown in orange. \label{fig:tgg}}
%    \vspace{-0.3cm}
%\end{wrapfigure}
\end{figure}
\begin{figure}[h]
	\centering
	\subfigure[n:5 |U|:10 r:8]{
		\includegraphics[width=0.23\columnwidth]{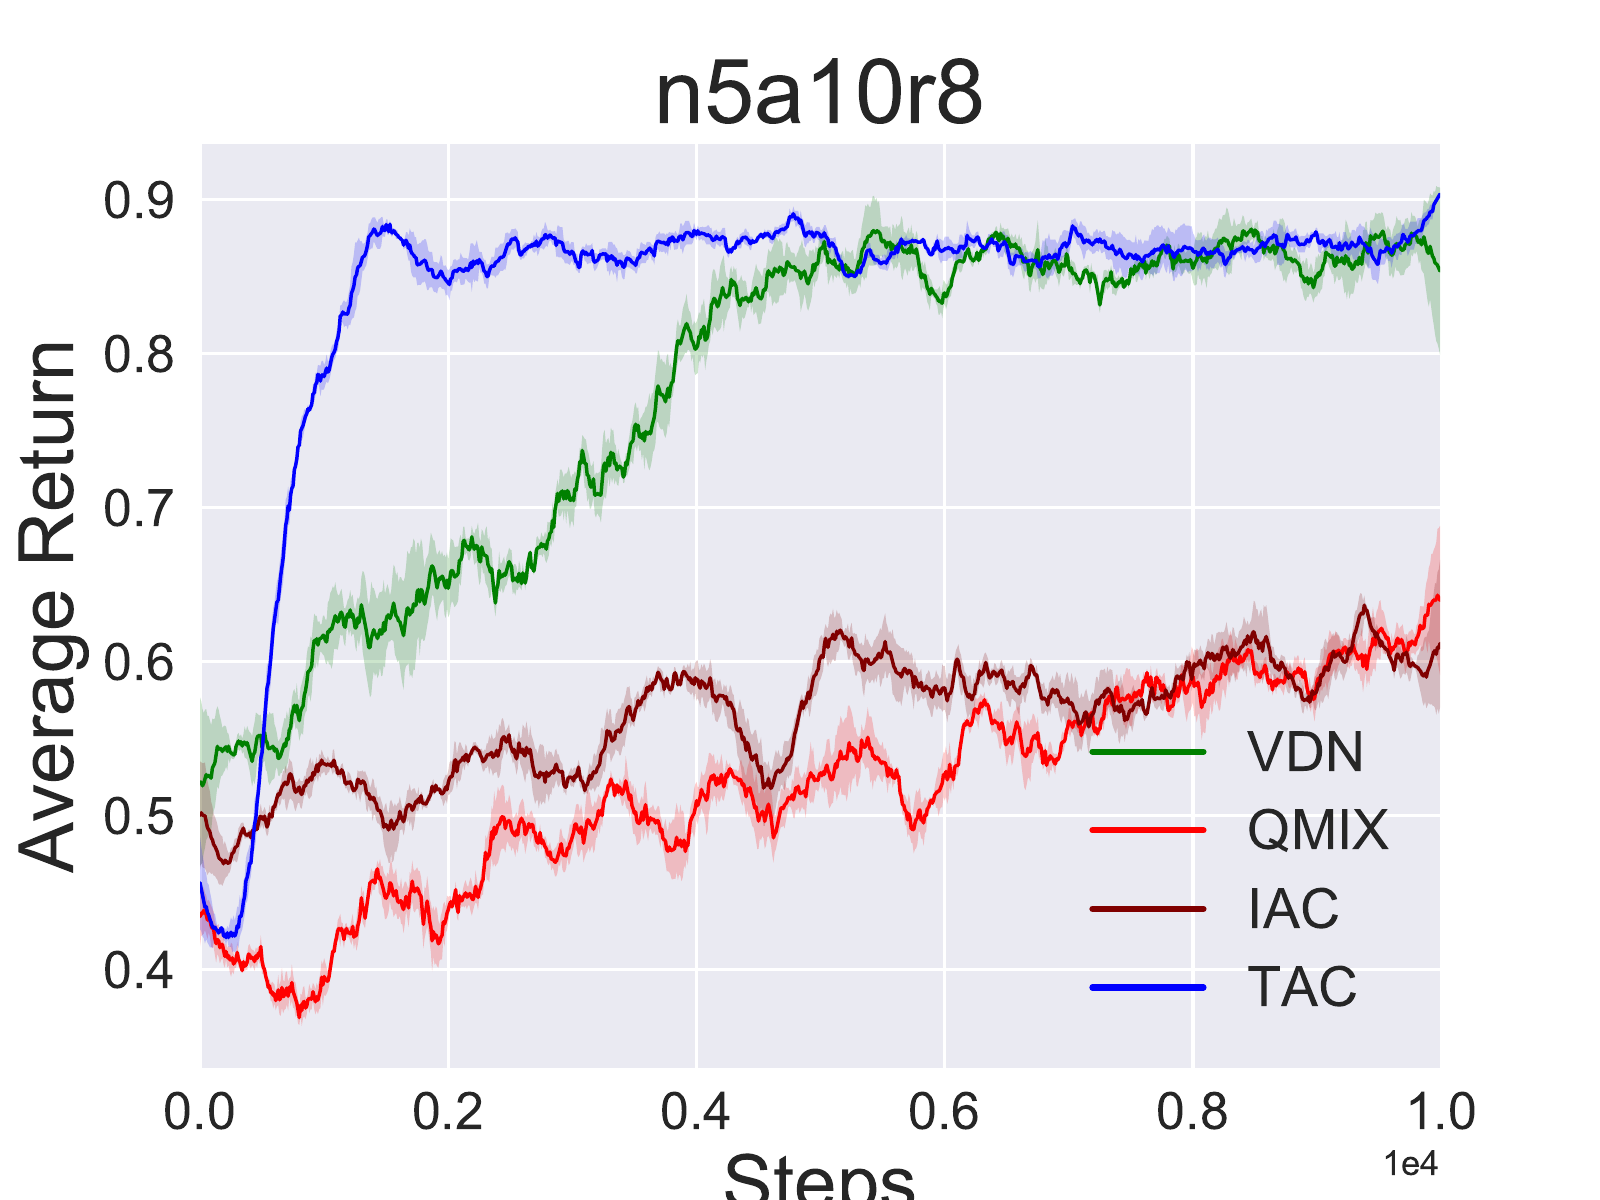}\label{fig:n5a10}}
	\subfigure[n:6 |U|:10 r:8]{
		\includegraphics[width=0.23\columnwidth]{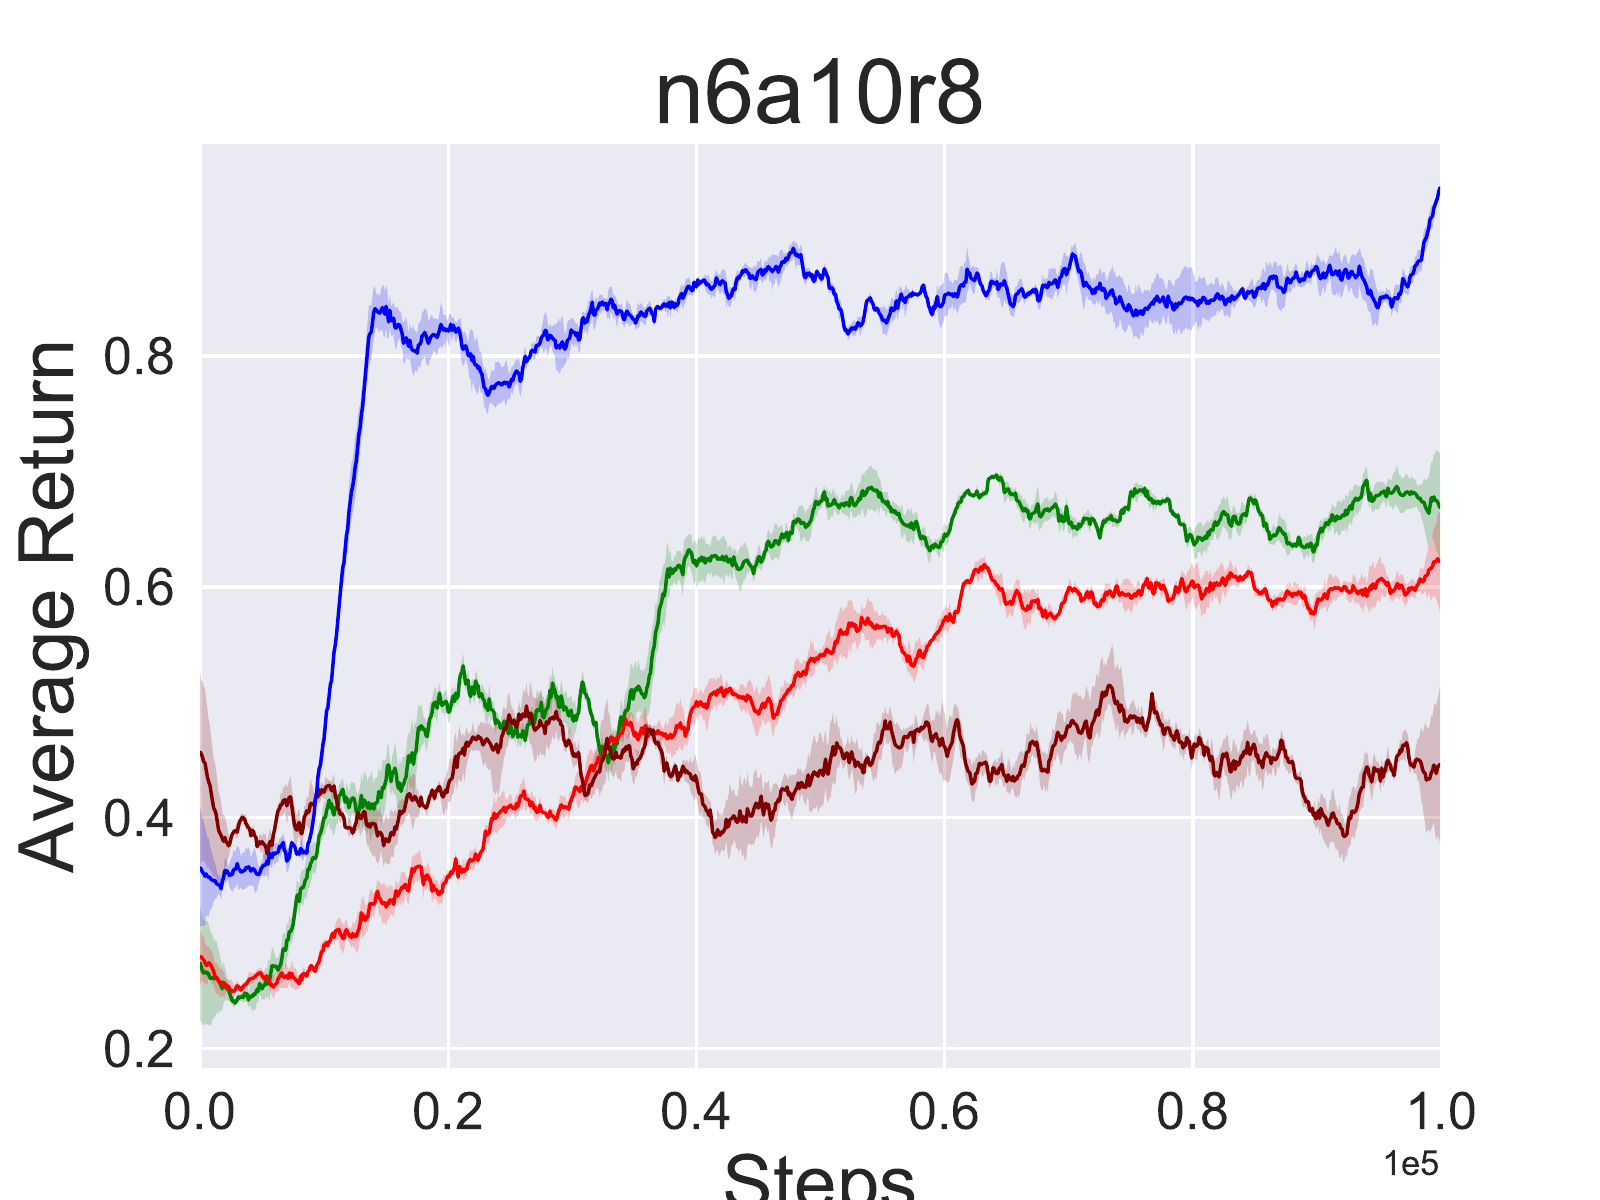}\label{fig:n6a10}}
	\subfigure[Dependence on approximation rank]{
		\includegraphics[width=0.23\columnwidth]{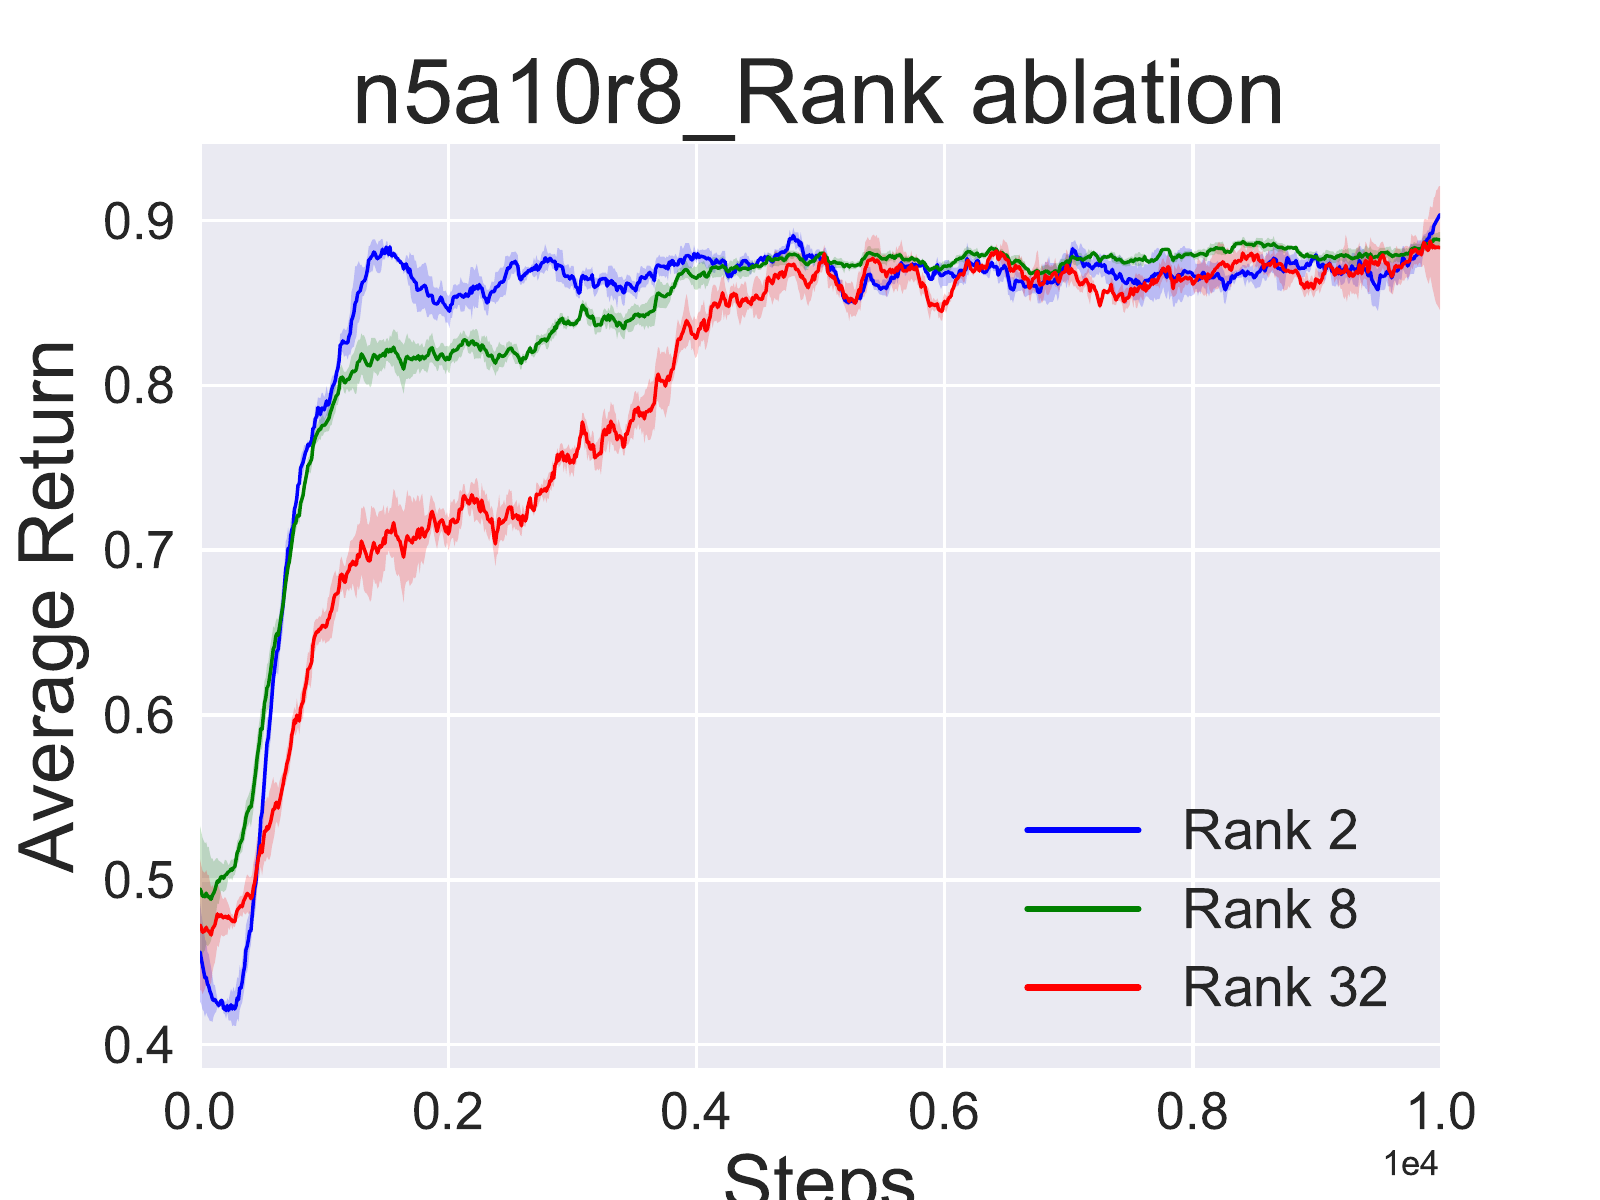}\label{fig:rab}}
	\subfigure[Effects of approximation]{
		\includegraphics[width=0.23\columnwidth]{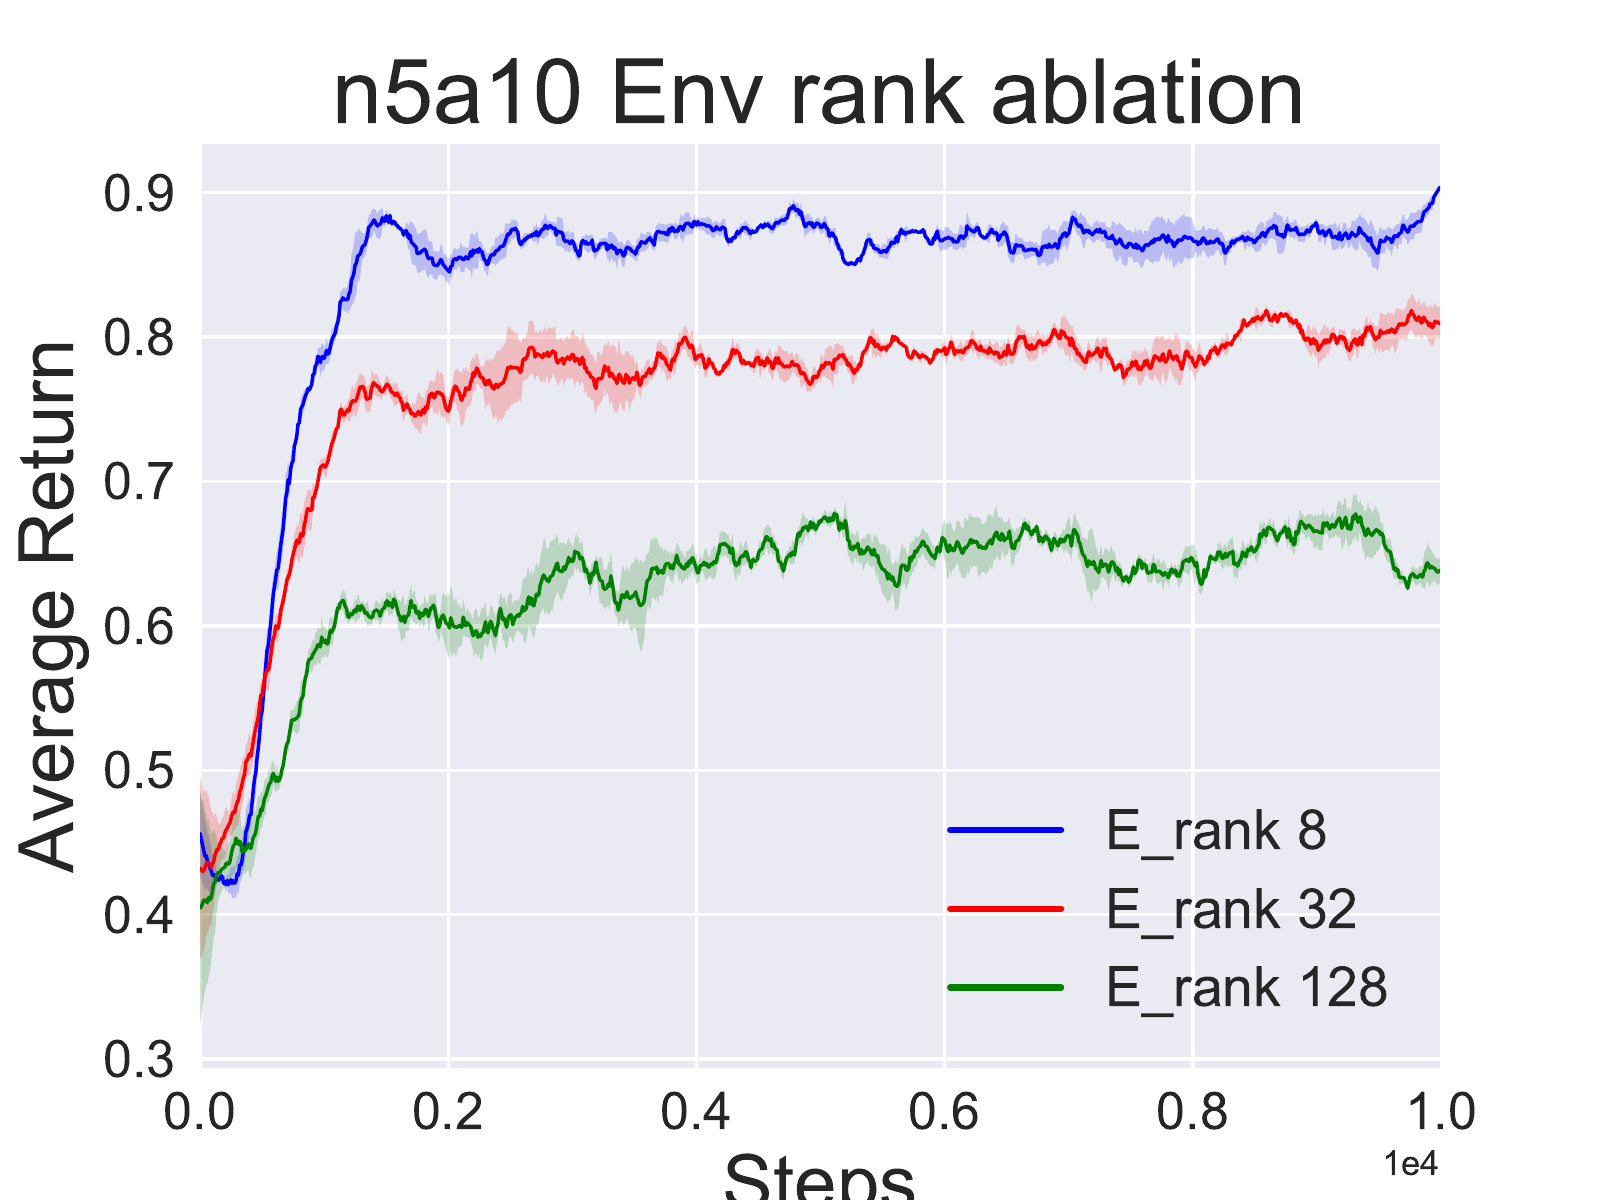}\label{fig:erab}}
	\caption{Experiments on tensor games.}
	\vspace{-0.5cm}
\end{figure}

\cref{fig:n5a10} \cref{fig:n6a10} present the learning curves for the algorithms for two game scenarios, averaged over 5 random runs with game parameters as mentioned in the figures. We observe that \textsc{Tesseract} outperforms the other algorithms in all cases. Moreover, while the other algorithms find it increasingly difficult to learn good policies, \textsc{Tesseract} is less affected by this increase in action space. As opposed to the IAC baseline, \textsc{Tesseract} quickly learns an effective low complexity critic for scaling the policy gradient. QMIX performs worse than VDN due to the additional challenge of learning the mixing network.

In \cref{fig:rab} we study the effects of increasing the approximation rank of Tesseract ($k$ in decomposition $\hat Q(s) \approx T = \sum_{r=1}^k w_r\otimes^n g_{\phi,r}(s^i) ,i \in \{1..n\},$) for a fixed environment with $5$ agents, each having $10$ actions and the environment rank being $8$. While all the three settings learn the optimal policy, it can be observed that the number of samples required to learn a good policy increases as the approximation rank is increased (notice delay in 'Rank 8', 'Rank 32' plot lines). This again is in-line with our PAC results, and makes intuitive sense as a higher rank of approximation directly implies more parameters to learn which increases the samples required to learn. 

We next study how approximation of the actual $Q$ tensors affects learning. In \cref{fig:erab} we compare the performance of using a rank-$2$ \textsc{Tesseract} approximation for environment with $5$ agents, each having $10$ actions and the environment reward tensor rank being varied from $8$ to $128$. We found that for the purpose of finding the optimal policy, \textsc{Tesseract} is fairly stable even when the environment rank is greater than the model approximation rank. However performance may drop if the rank mismatch becomes too large, as can be seen in \cref{fig:erab} for the plot lines 'E\_rank 32', 'E\_rank 128', where the actual rank required to approximate the underlying reward tensor is too high and using just $2$ factors doesn't suffice to accurately represent all the information.  

\subsubsection{Experimental setup for Tensor games}

For tensor game rewards, we sample $k$ linearly independent vectors $u_r^i$ from $|\mathcal{N}(0,1)^{|U|}|$ for each agent dimension $i \in \{1..n\}$. The reward tensor is given by $T=\sum_{r=1}^k w_r\otimes^n u_r^i ,i \in \{1..n\}$. Thus $T$ has roughly $k$ local maxima in general for $k<<|U|^n$. We normalise $\hat T$ so that the maximum entry is always $1$. 

All the agents use feed-forward neural networks with one hidden layer having $64$ units for various components. Relu is used for non-linear activation.

The training uses ADAM \citep{kingma2014adam} as the optimiser with a $L2$ regularisation of $0.001$. The learning rate is set to $0.01$. Training happens after each environment step.

The batch size is set to $32$. For an environment with $n$ agents and $a$ actions available per agent we run the training for $\frac{a^n}{10}$ steps. 

For VDN \citep{sunehag_value-decomposition_2017} and QMIX\citep{rashid2018qmix} the $\epsilon$-greedy coefficient is annealed from $0.9$ to $0.05$ at a linear rate until half of the total steps after which it is kept fixed.

For Tesseract ('TAC') and Independent Actor-Critic ('IAC') we use a learnt state baseline for reducing policy gradient variance. We also add entropy regularisation for the policy with coefficient starting at $0.1$ and halved after every $\frac{1}{10}$ of total steps.

We use an approximation rank of $2$ for Tesseract ('TAC') in all the comparisons except \cref{fig:rab} where it is varied for ablation.
