# Supplementary material for: Reinforcement Learning in Factored Action Spaces using Tensor Decompositions
Source: arXiv:2110.14538 source file (2021-10-27)
Supplement: Supplementary file 2 [file appendix_proofs.tex]

\section{Additional Proofs}
\addtocounter{theorem}{-2}
\addtocounter{proposition}{-1}
\addtocounter{lemma}{-1}
\label{app:proofs}
\subsection{Proof of \cref{thm:debound}}
\label{proof:app_dbound}

\begin{theorem}[Model based estimation of $\hat R, \hat P$ error bounds]
Given any $\epsilon>0, 1>\delta>0$, for a policy $\pi$ with the policy tensor satisfying $\pi(\mathbf{u}|s)\geq \Delta$, where
\begin{align}
\label{eq:polcon}
\Delta = \max_s 
\frac{C_1 \mu_{s}^6 k^5 (w_{s}^{\text{max}})^4 \log(|U|)^4 \log(3k||R(s)||_{F}/\epsilon)}
{|U|^{n/2} (w_{s}^{\text{min}})^4}  
\end{align}
and $C_1$ is a problem dependent positive constant. There exists $N_0$ which is $O(|U|^{\frac{n}{2}})$ and polynomial in $\frac{1}{\delta},\frac{1}{\epsilon}, k$ and relevant spectral properties of the underlying MDP dynamics such that for samples $\geq N_0$, we can compute the estimates $\bar R(s), \bar P(s,s')$ such that w.p. $\geq 1-\delta$, $||\bar{R}(s)-\hat R(s)||_F\leq \epsilon, ||\bar{P}(s,s')-\hat P(s,s')||_F\leq \epsilon, \forall s,s' \in S$.
\end{theorem}
% \begin{proof}
% See \cref{proof:debound}
% \end{proof}
\begin{proof}
For the simplicity of notation and emphasising key points of the proof, we focus on orthogonal symmetric tensors with $n=3$. Guidelines for more general cases are provided by the end of the proof. 

We break the proof into three parts:
Let policy $\pi$ satisfy $\pi(\mathbf{u}|s)\geq \Delta$ \cref{eq:polcon}. Let $\rho$ be the stationary distribution of $\pi$ (exists by \cref{a3}) and let $N_1  = \max_s \frac{1}{\rho(s)}\log\Big(\frac{12\sqrt{k}||R(s)||_F}{\epsilon}\Big)$. From $N_1$ samples drawn from $\rho$ by following $\pi$, we estimate $\bar{R}$, the estimated reward tensor computed by using Algorithm $1$ in \cite{jain2014provable}. We have by application of union bound along with Theorem $1.1$ in \cite{jain2014provable} for each $s\in S$, w.p. $\geq 1 - |U|^{-5}\log_2\Big(\frac{12\sqrt{k}\prod_s||R(s)||_F}{\epsilon}\Big) = p_\epsilon$, $||\bar{R}(s)-\hat R(s)||_F\leq \epsilon/3, \forall s\in S$. We now provide a boosting scheme to increase the confidence in the estimation of $\hat R(\cdot)$ from $p_\epsilon$  to $1 - \delta/3$. Let $\eta = \frac{1}{2}\Big(p_\epsilon -\frac{1}{2}\Big) > 0$ (for clarity of the presentation we assume $p_\epsilon >\frac{1}{2}$ and refer the reader to \cite{kearns1994introduction} for the other more involved case). We compute $M$ independent estimates $\{\bar R_i, i \in \{1..M\}\}$ for $\hat R(s)$ and find the biggest cluster $\mathcal{C} \subseteq \{\bar R_i\}$ amongst the estimates such that for any $\bar R_i, \bar R_j \in \mathcal{C}, ||\bar R_i-\bar R_j||_F \leq \frac{2\epsilon}{3}$. We then output any element of $\mathcal{C}$. Intuitively as $p_\epsilon >\frac{1}{2}$, most of the estimates will be near the actual value $\hat R(s)$, this can be confirmed by using the Hoeffding Lemma\cite{kearns1994introduction}. It follows that for $M\geq \frac{1}{2\eta^2}\ln(\frac{3|S|}{\delta})$ the output of the above procedure satisfies $||\bar{R}(s)-\hat R(s)||_F\leq \epsilon$ w.p. $\geq 1 - \frac{\delta}{3|S|}$ for any particular $s$. Thus $MN_1$ samples from stationary distribution are sufficient to ensure that for all $s \in S$, w.p. $\geq 1 - \delta/3$, $||\bar{R}(s)-\hat R(s)||_F\leq \epsilon$.

Secondly we note that $\hat P (s,s')$ for any $s,s' \in S$ is a tensor whose entries are the parameters of a Bernoulli distribution. Under \cref{a2}, it can be seen as a latent topic model \cite{anandkumar2012method} with $k$ factors, $\hat P(s,s') = \sum_{r=1}^{k} w_{s,s',r}\otimes^n u_{s,s',r} $. Moreover it satisfies the conditions in Theorem $3.1$ \cite{anandkumar2012method} so that $\exists N_2  = \max_{s,s'}\frac{1}{\rho(s)} N_2(s,s')$ where each $N_2(s,s')$ is $\mathcal{O}\Big(\frac{k^{10} |S|^2 \ln^2(3|S|/\delta)}{\delta^2 \epsilon^{'2}}\Big)$ depending on the spectral properties of $\hat P(s,s')$ as given in the theorem and satisfies $||\bar{u_{s,s',r}}-u_{s,s',r}||_2\leq \epsilon'$ on running Algorithm B in \cite{anandkumar2012method} w.p. $\geq 1 - \frac{\delta}{3|S|}$. We pick $\epsilon' = \frac{\epsilon}{7n^2k \mu_{s,s'}^2 (w_{s,s'}^{\text{max}})^2} $ so that $||\bar{P}(s,s')-\hat P(s,s')||_F\leq \epsilon, \forall s,s' \in S$. We filter off the effects of sampling from a particular policy by using lower bound constraint in \cref{eq:polcon} and sampling $\frac{N_2}{\Delta}$ samples.

Finally we account for the fact that there is a delay in attaining the stationary distribution $\rho$ and bound the failure probability of significantly deviating from $\rho$ empirically. Let $\rho' = \min_s \rho(s)$ and $t_{\text{mix},\pi}(x)$ represent the minimum number of samples that need to drawn from the Markov chain formed by fixing policy $\pi$ so that for the state distribution $\rho_{t}(s)$ at time step $t = t_{\text{mix},\pi}(x)$ we have $TV(\rho_{t} - \rho)\leq x$ for any starting state $s\in S$ where $TV(\cdot,\cdot)$ is the total variation distance. We let the policy run for a burn in period of $t'=t_{\text{mix},\pi}(\rho'/4)$. For a sample of $N_3$ state transitions after the burn in period, let $\bar \rho$ represent the empirical state distribution. By applying the Hoeffding lemma for each state, we get: $P(|\bar\rho(s) - \rho_{t'}(s)|\geq \rho'/4)\leq 2\exp\Big(\frac{-N_3\rho^{'2}}{8}\Big)$, so that for $N_3\geq \frac{8}{\rho^{'2}}\ln\Big(\frac{6|S|}{\delta}\Big)$ we have w.p. $\geq 1 - \frac{\delta}{3|S|}$, $|\bar\rho(s) - \rho(s)|< \rho'/2, \forall s \in S$.

Putting everything together we get with $t_{\text{mix},\pi}(\rho'/4) + \max\{2MN_1, \frac{2N_2}{\Delta}, N_3\}$ samples, the underlying reward and probability tensors can be recovered such that w.p. $\geq 1-\delta$, $||\bar{R}(s)-\hat R(s)||_F\leq \epsilon, ||\bar{P}(s,s')-\hat P(s,s')||_F\leq \epsilon, \forall s,s' \in S$.

For extending the proof to the case of non-orthogonal tensors, we refer the reader to use whitening transform as elucidated in \cite{anandkumar2014tensor}. Likewise for asymmetric, higher order ($n>3$) tensors methods shown in \cite{jain2014provable, anandkumar2014tensor, anandkumar2012method} should be used. Finally for the case of M-POMDP and M-ROMDP, the corresponding results for single agent POMDP and ROMDP should be used, as detailed in \cite{azizzadenesheli2019reinforcement, azizzadenesheli2016reinforcement} respectively. 
\end{proof}

\subsection{Proof of \cref{tvbound}}
\label{proof:tvbound}
\begin{lemma}
For transition tensor estimates satisfying $||\bar{P}(s,s')-\hat P(s,s')||_F\leq \epsilon$, we have for any given state and action pair $s,a$, the distribution over the next states follows: $TV(P'(\cdot|s,a),P(\cdot|s,a))\leq \frac{1}{2}(|1-f|+f|S|\epsilon)$ where $\frac{1}{1+\epsilon|S|}\leq f \leq\frac{1}{1-\epsilon|S|}$. Similarly for any policy $\pi$, $TV(\bar P_{\pi}(\cdot|s),P_{\pi}(\cdot|s)), TV(\bar P_{\pi}(s',a'|s),P_{\pi}(s',a'|s))\leq \frac{1}{2}(|1-f|+f|S|\epsilon)$ 
\end{lemma}
\begin{proof}
Let $ \bar P(\cdot|s,a)$ be the next state probability estimates obtained from the tensor estimates. We next normalise them across the next states to get the (estimated)distribution $ P'(\cdot|s,a) = f \bar P(\cdot|s,a)$ where $f = \frac{1}{\sum_{s'}\bar P(s'|s,a)}$. Dropping the conditioning for brevity we have:
\begin{align}
TV(P',P) &= \frac{1}{2}\sum_{s'} |P(s')-f \bar P(s')|\\
&\leq\frac{1}{2}(\sum_{s'} |P(s')-f P(s')| +|f P(s')- \bar P(s')|)\\
&=\frac{1}{2}(|1-f|+f|S|\epsilon) 
\end{align}
The other two results follow using the definition of TV and Fubini's theorem followed by reasoning similar to above.
\end{proof}

\subsection{Proof of \cref{thm:q_err}}
\label{proof:app_q_err}
\begin{theorem}
[Error bound on policy evaluation]
Given a behaviour policy $\pi_b$ satisfying the conditions in \cref{thm:debound} and being executed for steps $\geq N_0$, we have that for any policy $\pi$ the model based policy evaluation $Q_{\bar P,\bar R}^\pi$ satisfies:
\begin{align}
|Q_{P,R}^\pi(s,a) - Q_{\bar P,\bar R}^\pi(s,a)|&\leq (|1-f|+f|S|\epsilon)\frac{\gamma}{2(1-\gamma)^2}+   \frac{\epsilon}{1-\gamma}, \forall (s,a)\in S\times U^n
\end{align} 
where $f$ is as defined in \cref{tvbound}.
\end{theorem}
\begin{proof}
Let $\bar P, \bar R$ be the estimates obtained after running the procedure as described in \cref{thm:debound} with samples corresponding to error $\epsilon$ and confidence $1-\delta$. We will bound the error incurred in estimation of the action-values using $\bar P, \bar R$. We have for any $\pi$ by using triangle inequality 
\begin{align}
\label{tring_q}
|Q_{P,R}^\pi(s,a) - Q_{\bar P,\bar R}^\pi(s,a)|&\leq |Q_{P,R}^\pi(s,a)- Q_{\bar P, R}^\pi(s,a)| + |Q_{\bar P, R}^\pi(s,a) - Q_{\bar P,\bar R}^\pi(s,a)|   
\end{align}
where we use the subscript to denote whether actual or approximate values are used for $P,R$ respectively. We first focus on the first term on the RHS of \cref{tring_q}. Let $R_\pi(s_t) = \sum_{a_t} \pi(a_t|s_t) R(s_t,a_t)$. We use $P_{t,\pi}(\cdot|s) = (P_{\pi}(\cdot|s))^t$ to denote the state distribution after $t$ time steps. Consider a horizon $h$ interleaving $Q$ estimate given by:
\begin{align}
Q_h^\pi(s,a) &= R(s_t,a_t)+\sum_{t=1}^{h-1}\gamma^t\mathbb{E}_{\bar P_{t,\pi}(\cdot|s)}[ R_\pi(s_t)]+ \sum_{t=h}^{\infty}\gamma^t\mathbb{E}_{P_{t-h,\pi}(\cdot|s_h)\cdot \bar P_{h,\pi}(s_h|s) }[ R_\pi(s_t)]
\end{align}
Where $s_0=s, a_0=a$ and the first $h$ steps are unrolled according to $\bar P_\pi$, the rest are done using the true transition $P_\pi$. We have that:
\begin{align}
|Q_{P,R}^\pi(s,a) - Q_{\bar P, R}^\pi(s,a)|&=|Q_0^\pi(s,a) - Q_\infty^\pi(s,a)|\leq \sum_{h=0}^\infty |Q_h^\pi(s,a) - Q_{h+1}^\pi(s,a)|
\end{align}
Each term in the RHS of the above can be independently bounded as : 
\begin{align}
|Q_h^\pi(s,a) - Q_{h+1}^\pi(s,a)|=&\gamma^{h+1}\Big|\mathbb{E}_{\bar P_{h+1,\pi}(s_{h+1}|s)}\Big[\sum_{a_{h+1}}\pi(a_{h+1}|s_{h+1})Q_\infty^\pi(s_{h+1}.a_{h+1})\Big]\\&-\mathbb{E}_{P_\pi\bar P_{h,\pi}(s_{h+1}|s)}\Big[\sum_{a_{h+1}}\pi(a_{h+1}|s_{h+1})Q_\infty^\pi(s_{h+1}.a_{h+1})\Big]\Big|
\end{align}
As the rewards are bounded we get the expression above is $\leq \frac{1}{1-\gamma}\gamma^{h+1}TV(\bar P_{\pi}(s',a'|s),P_{\pi}(s',a'|s))$. Finally using \cref{tvbound} we get $\leq (\frac{1}{2}(|1-f|+f|S|\epsilon))\frac{\gamma^{h+1}}{1-\gamma}$. And plugging in the original expression: 
\begin{align}
|Q_{P,R}^\pi(s,a) - Q_{\bar P, R}^\pi(s,a)|\leq (|1-f|+f|S|\epsilon)\frac{\gamma}{2(1-\gamma)^2}
\end{align}
Next the second term on the RHS of \cref{tring_q} can easily be bounded by $\frac{\epsilon}{1-\gamma}$ which gives:
\begin{align}
|Q_{P,R}^\pi(s,a) - Q_{\bar P,\bar R}^\pi(s,a)|&\leq (|1-f|+f|S|\epsilon)\frac{\gamma}{2(1-\gamma)^2}+   \frac{\epsilon}{1-\gamma}
\end{align}
\end{proof}

\vspace{-0.5cm}
\section{Discussion}
\subsection{Relation to other methods}
\label{discussion:vdn}
In this section we study the relationship between \textsc{Tesseract} and some of the existing methods for MARL.

\subsubsection{FQL}
FQL~\citep{chen2018factorized} uses a learnt inner product space to represent the dependence of joint Q-function on pair wise agent interactions. The following result shows containment of FQL representable action-value function by \textsc{Tesseract} : 
\begin{proposition}
The set of joint Q-functions representable by FQL is a subset of that representable by \textsc{Tesseract}.
\end{proposition}
\begin{proof}
In the most general form, any join Q-function representable by FQL has the form:
\begin{equation}
Q_{fql}(s, \mathbf{u}) = \sum_{i=1:n} q_i(s,u_i) + \sum_{i=1:n, j<i} \langle f_i(s,u_i), f_j(s,u_j) \rangle
\end{equation}
where $q_i: S\times U \to \mathbb{R}$ are individual contributions to joint Q-function and $f_i: S\times U \to \mathbb{R}^d$ are the vectors describing pairwise interactions between the agents. There are $n \choose 2$ pairs of agents to consider for (pairwise)interactions. Let $\mathscr{P} \triangleq {(i,j)}$ be the ordered set of agent pairs where $i>j$ and $i,j \in \{1..n\}$, let $\mathscr{P}_{k}$ denote the $k$th element of $\mathscr{P}$. Define membership function $m:\mathscr{P} \times \{1..n\} \to \{0,1\}$ as: 
\begin{align}
    m((i,j),x) =
    \begin{cases*}
      1     & if $x=i \vee x=j$ \\
      0     & otherwise
    \end{cases*}
\end{align}
Define the mapping $v_i: S \to \mathbb{R}^{|U|\times D}$ where $D = d {n \choose 2}+n$ and $v_{i,k}$ represents the $k$th column of $v_i$. 
\begin{align}
    v_i(s) \triangleq
    \begin{cases*}
      v_i(s)[j, (k-1)d+1:kd] = f_i(s, u_j)     & if $m(\mathscr{P}_{k}, i)=1$ \\
      v_i(s)[j, D-n+i] = q_i(s, u_j)\\
      v_i(s)[j, k] = 1     & otherwise
    \end{cases*}
\end{align}
We get that the tensors:
\begin{equation}
Q_{fql}(s) = \sum_{k=1}^D \otimes^n v_{i,k}(s)
\end{equation}
Thus any $Q_{fql}$ can be represented by \textsc{Tesseract}, note that the converse is not true ie. any arbitrary Q-function representable by \textsc{Tesseract} may not be representable by FQL as FQL cannot model higher-order ($>2$ agent) interactions. A simple example of this is the one-hot tensor describing the joint action-values $Q_{3,2}$ for a single state MMDP with $3$ agents and $2$ actions per agent, having entries $Q_{3,2}(1,1,1) = 1$ and $Q_{3,2}(i,j,k)=0, \forall i,j,k \in\{0,1\} \wedge i+j+k<3$, we have that $\forall d \in \mathbb{N}, \nexists f_i$ for which $Q_{3,2}$ can be expressed as sum of pairwise inner products. 
\end{proof}

\subsubsection{VDN}
VDN~\cite{sunehag_value-decomposition_2017} learns a decentralisable factorisation of the joint action-values by expressing it as a sum of per agent utilities $\hat Q=\oplus^n u_i ,i \in \{1..n\}$. This can be equivalently learnt in \textsc{Tesseract} by finding the best rank one projection of $\exp(\hat Q(s))$. We formalise this in the following result: 
\begin{proposition}
\label{prop:vdn}
For any MMDP, given policy $\pi$ having $Q$ function representable by VDN  ie. $\hat Q^{\pi}(s)=\oplus^n u_i(s) ,i \in \{1..n\}$, $\exists v_i(s) \forall s\in S$, the utility factorization can be recovered from rank one CP-decomposition of $\exp(\hat Q^{\pi})$
\end{proposition}
\begin{proof}
We have that :
\begin{align}
\exp(\hat Q^{\pi}(s)) &= \exp(\oplus^n u_i(s))\\
&=\otimes^n \exp(u_i(s))
\end{align}
Thus $(\exp(u_i(s)))_{i=1}^n \in \argmin_{v_i(s)}||\exp(\hat Q^{\pi}(s)) - \otimes^n v_i(s)||_F \forall s \in S$ and there always exist $v_i(s)$ that can be mapped to some $u_i(s)$ via exponentiation.
In general any Q-function that is representable by VDN can be represented by \textsc{Tesseract} under an exponential transform  (\cref{subsec:TessAlgos}).
\end{proof}

\subsection{Injecting Priors for Continuous Domains}
\label{app:cenv}
\begin{figure}[h]
\centering
\includegraphics[width=0.4\linewidth]{figures/pp_perturb.png}
\caption{Continuous actions task with three agents chasing a prey. Perturbing Agent 2's action direction by small amount $\theta$ leads to a small change in the joint value. \label{fig:perturb}}
\end{figure}

We now discuss the continuous action setting. Since the action set of each agent is infinite, we impose further structure while maintaining appropriate richness in the hypothesis class of the proposed action value functions. Towards this we present an example of a simple prior for \textsc{Tesseract} for continuous action domains. WLOG, let $U\triangleq \mathbb{R}^d$ for each agent $\in {1..n}$. We are now interested in the function class given by $\mathcal{Q}\triangleq \{Q: S\times U^n\to \mathbb{R}\}$ where each $Q(s)$ $\triangleq \langle T(s,\{||u^i||_2\}), \otimes^n u^i\rangle$, here $T(\cdot): S\times \mathbb{R}^n\to \mathbb{R}^{d^n}$ is a function that outputs an order $n$ tensor and is invariant to the direction of the agent actions, $\langle\cdot,\cdot\rangle$ is the dot product between two order $n$ tensors and  $||\cdot||_2$ is the Euclidean norm. Similar to the discrete case, we define 
$\mathcal{Q}_k \triangleq \{Q: Q\in \mathcal{Q} \land rank(T(\cdot)) =k, \forall s \in S\}$. The continuous case subsumes the discrete case with $T(\cdot)\triangleq Q(\cdot)$ and actions encoded as one hot vectors. We typically use rich classes like deep neural nets for $Q$ and $T$ parametrised by $\phi$.

We now briefly discuss the motivation behind the example continuous case formulation: for many real world continuous action tasks the joint payoff is much more sensitive to the magnitude of the actions than their directions, i.e., slightly perturbing the action direction of one agent while keeping others fixed changes the payoff by only a small amount (see \cref{fig:perturb}). Furthermore, $T_\phi$ can be arbitrarily rich and can be seen as representing utility per agent per action dimension, which is precisely the information required by methods for continuous action spaces that perform gradient ascent w.r.t.\ $\nabla_{u^i}Q$ to ensure policy improvement. Further magnitude constraints on actions can be easily handled by a rich enough function class for $T$. Lastly we can further abstract the interactions amongst the agents by learnable maps $f_\eta^i(u^i,s): \mathbb{R}^d \times S \to \mathbb{R}^m$, $m>>d$ and considering classes  $Q(s,\mathbf{u})\triangleq \langle T(s,\{||u^i||\}), \otimes^n f_\eta^i(u^i)\rangle$ where $T(\cdot): S\times \mathbb{R}^n\to \mathbb{R}^{m^n}$. 

\subsection{Additional theoretical discussion}
\label{app:atd}
\subsubsection{Selecting the CP-rank for approximation}
While determining the rank of a fully observed tensor is itself NP-hard \citep{hillar2013most}, we believe we can help alleviate this problem due to two key observations:
\begin{itemize}
    \item The tensors involved in \textsc{Tesseract} capture dependence of transition and reward dynamics on the action space. Thus if we can approximately identify (possibly using expert knowledge) the various aspects in which the actions available at hand affect the environment, we can get a rough idea of the rank to use for approximation.
    \item Our experiments on different domains (\cref{sec:exps}, \cref{app:additional_exp}) provide evidence that even when using a rank insufficient approximation, we can get good empirical performance and sample efficiency. (This is also evidenced by the empirical success of related algorithms like VDN which happen to be specific instances under the \textsc{Tesseract} framework.)
\end{itemize}
